# Supplementary material for: Optimisation of amplification and gas mixture for directional Dark Matter searches with the CYGNO/INITIUM project
Source: arXiv:2507.02474 source file (2025-07-03)
Supplement: Supplementary file 1 [file Appendix_D.pdf]

# C-Mount Mega-Pixel Lens

**Xenon 0.95/25-0037**

This 1“ megapixel lens has an extremely high relative aperture of 0.95, making it perfectly suitable for low light applications. The lens is corrected and coated for the visible light in the range of 400 - 700 nm. Even under production and / or extreme conditions, the robust mechanical design with lockable focus and iris setting mechanism guarantees reliable continuous use in which the set optical parameters remain in place.

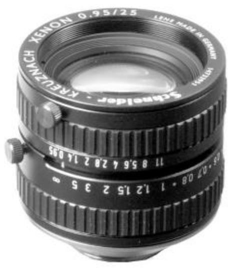

Xenon 0.95/25

**Key Features**

- Very high relative aperture of 0.95
- Complex optical design
- High optical imaging performance
- Compact full metal mount
- Vibration insensitivity for stable imaging performance
- Focus and iris setting lockable

**Applications**

- Machine Vision and other imaging applications
- 3D measurement
- Traffic
- Medical
- Robot vision
- Food processing

**Technical Specifications**

| | |
|---|---|
| F-number | 0.95 |
| Focal length | 25.6 mm |
| Image circle | 16 mm |
| Transmission | 400 - 700 nm |
| Interface | C-Mount |
| Weight | 240 gr. |
| Filter tread | M39 x 0.5 |
| Code no. | 12101 |

# Xenon 0.95/25

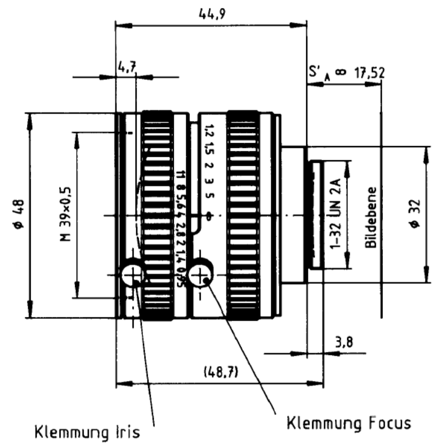


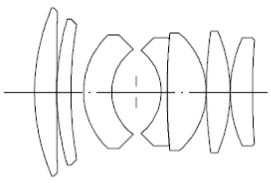

XENON 0.95/25MM

| | | | |
|---|---|---|---|
| $f'$ = 25.6 mm | $\beta'_p$ = 4.086 |
| $s_F$ = 16.9 mm | $s_{EP}$ = 23.1 mm |
| $s'_{F'}$ = 16.2 mm | $s'_{AP}$ = -88.5 mm |
| $HH'$ = -10.5 mm | $\Sigma d$ = 41.4 mm |

XENON 0.95/25MM

MODULATION with reference to the relative image height

| | | | | | | | |
|---|---|---|---|---|---|---|---|
| Wavelength λ [nm] : | 555 | 655 | 605 | 505 | 455 | 405 |
| Spectral weighting [%] : | 19.6 | 23.7 | 22.2 | 15.7 | 12.1 | 6.7 |
| Spatial frequency R [1/mm] : | 10 | 20 | 30 | | | |
| Format [mm X mm] : | 9.6 X 12.8 | | | | | |
| Diagonal 2u' [mm] : | 16.0 | | | | | |

radial ——
tangential — —

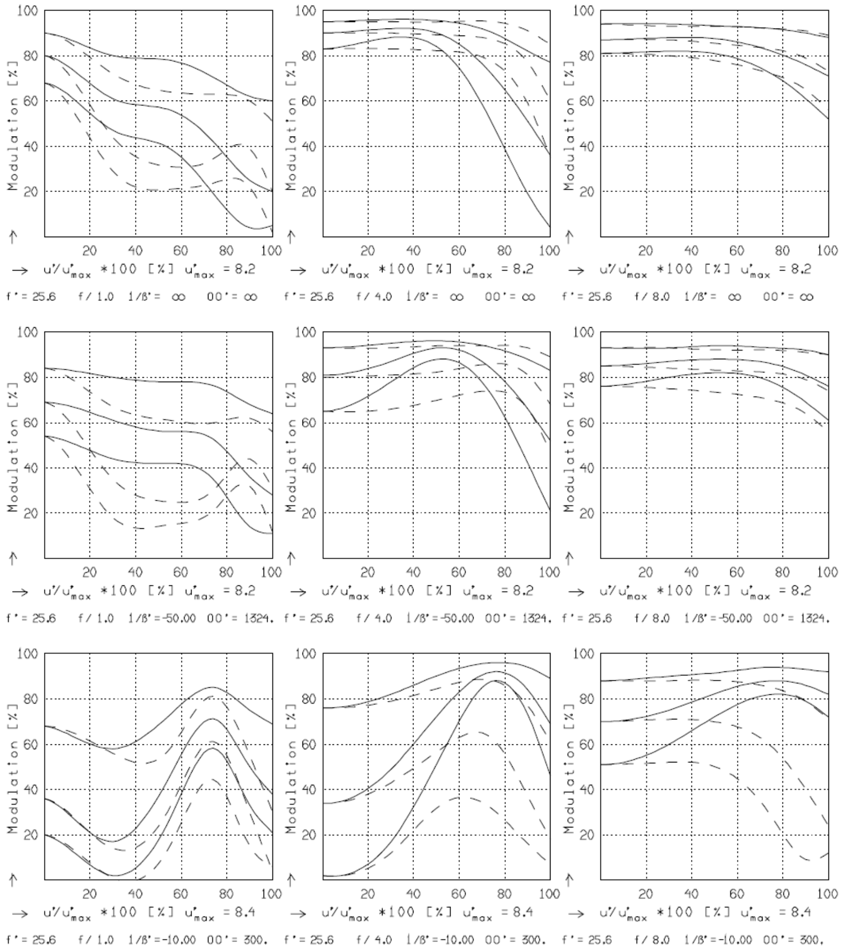


Focusing : $MTF_{max}$ at f / 1.0 , R = 30 1/mm, $u'/u'_{max}$ = 0

Schneider KREUZNACH

# Xenon 0.95/25

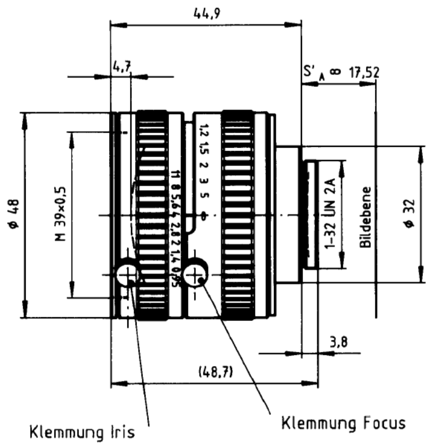


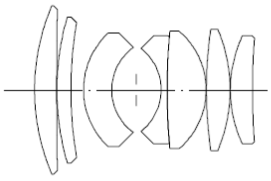

XENON 0.95/25MM

| | | | | | |
|---|---|---|---|---|---|
| f' | = 25.6 | mm | ß'p | = 4.086 | |
| $s_F$ | = 16.9 | mm | $s_{EP}$ | = 23.1 | mm |
| $s'_{F'}$ | = 16.2 | mm | $s'_{AP}$ | = -88.5 | mm |
| HH' | = -10.5 | mm | Σ d | = 41.4 | mm |

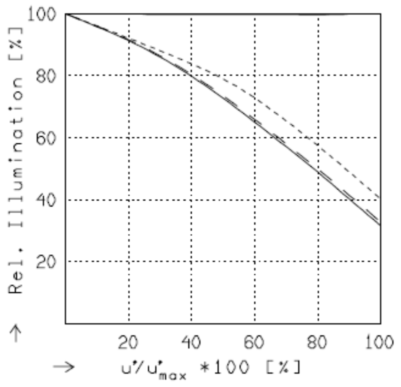


## RELATIVE ILLUMINATION

The relativ illumination is shown for the given focal distances or magnifications.

f / 1.0 f / 4.0 f / 8.0

| | | | |
|---|---|---|---|
| —— | ß' = 0.0000 | $u'_{max}$ = 8.0 | OO' = ∞ |
| — — | ß' = -0.0200 | $u'_{max}$ = 8.0 | OO' = 1323. |
| ----- | ß' = -0.1000 | $u'_{max}$ = 8.0 | OO' = 300. |

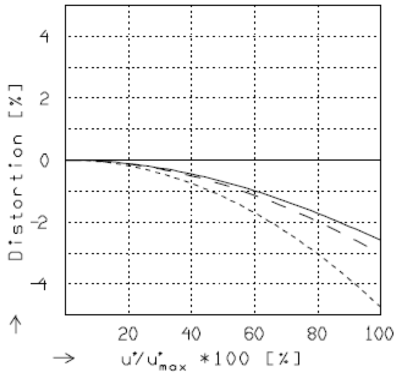


## DISTORTION

Distortion is shown for the given focal distances or magnifications. Positive values indicate pincushion distortion and negative values barrel distortion.

| | | | |
|---|---|---|---|
| —— | ß' = 0.0000 | $u'_{max}$ = 8.0 | OO' = ∞ |
| — — | ß' = -0.0200 | $u'_{max}$ = 8.0 | OO' = 1323. |
| ----- | ß' = -0.1000 | $u'_{max}$ = 8.0 | OO' = 300. |

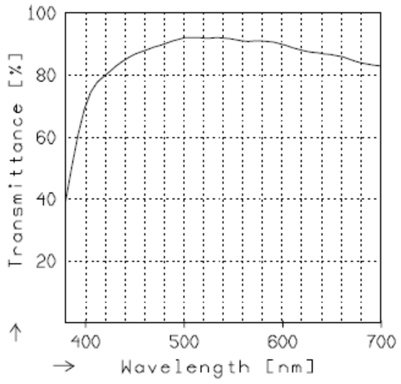


## TRANSMITTANCE

Relative spectral transmittance is shown with reference to wavelength.

OPT-SKR68-06/2018 · Subject to technical change without notice. No liability is accepted for errors which may be contained in this document.
